# Supplementary material for: MambaByte: Token-free Selective State Space Model
Source: arXiv:2401.13660 source file (2024-08-09)
Supplement: Supplementary file 1 [file d_parallel_scans.tex]

\section{Parallel scan for linear recurrences}
\label{app:scans}

The parallelization of scan operations has been well explored \cite{ladner1980parallel,lakshmivarahan1994parallel,blelloch1990prefix}, with several scientific computing libraries containing optimized routines. In this section, we detail the use of a parallel scan for linear recurrence in $\S\ref{sec:model}$ as a specific application of a more generalized setting in $\S1.4$ of \citet{blelloch1990prefix}.

To compute a linear recurrence $h[k] = \discrete{A}h[k-1] + \discrete{B}x[k]$ for a sequence of length $L$, let us define $L$ initial elements $e_{1:L}$, such that:
\begin{align}
\label{eq:scan-init}
    e_k = \left(A_k, b_k\right) \coloneqq \left(\discrete{A}, \discrete{B}x[k]\right),
\end{align}
where $A_k, \discrete{A} \in \R[n][n]$, $\discrete{B} \in \R[n][1]$, and $x[k], b_k \in \R[n]$. These initial $L$ elements are precomputed before the scan.

Now, the binary associative operator $\bullet$ to use on the linear recurrence is defined as:
\begin{align}
    \label{eq:recurrence-operator}
    e_j \bullet e_k \equiv (A_k A_j, A_k b_j + b_k).
\end{align}

\paragraph{Associativity of the operator.} Note that the binary operator shown above in (\ref{eq:recurrence-operator}) is associative:
\begin{align*}
    e_i \bullet (e_j \bullet e_k) &= e_i \bullet (A_kA_j, A_kb_j + b_k) \\
    &= ((A_kA_j)A_i, A_kA_jb_i + (A_kb_j + b_k)) \\
    &= (A_k(A_jA_i), A_k(A_jb_i + b_j) + b_k) \\
    &= (A_jA_i, A_jb_i + b_j) \bullet e_k \\
    &= (e_i \bullet e_j) \bullet e_k.
\end{align*}

\paragraph{Illustration of linear recurrence using the operator.} Using the binary associative operator in (\ref{eq:recurrence-operator}), we can see how the linear recurrence $h[k] = \discrete{A}h[k-1] + \discrete{B}x[k]$ can be computed. By setting $h[0] = 0$, we have:
\begin{align*}
    h[1] &= \discrete{B}x[1]; \\
    h[2] &= \discrete{A}\discrete{B}x[1] + \discrete{B}x[2]; \\
    h[3] &= \discrete{A}^2\discrete{B}x[1] + \discrete{A}\discrete{B}x[2] + \discrete{B}x[3]; \\
     &\vdots \\
    h[k] &= \discrete{A}^{k-1}\discrete{B}x[1] + \discrete{A}^{k-2}\discrete{B}x[2] + \dots + \discrete{A}\discrete{B}x[k-2] + \discrete{B}x[k-1].
\end{align*}

\begin{algorithm}[!ht]
    \begin{algorithmic}
        \Procedure{Reduce}{$[e_1, e_2, \dotsc, e_L]$, $\bullet$}
            \For{$d = 1, \dotsc, \log_2(L)$}
                \For{$i = 1, \dotsc, L$ in increments of $2^d$ \textbf{in parallel}}
                    \State $k \gets i + 2^d - 1$; $j \gets i + 2^{d - 1} - 1$ 
                    \State $e_k \gets e_j \bullet e_k$
                \EndFor
            \EndFor
        \EndProcedure
        \\
        \Procedure{DownSweep}{$[e_1, e_2, \dotsc, e_L]$, $\bullet$}
            \State {$e_L \gets (\I, 0)$}
            \For{$d = \log_2(L), \dotsc, 1$}
                \For{$i = 1, \dotsc, L$ in increments of $2^d$ \textbf{in parallel}}
                    \State $k \gets i + 2^d - 1$; $j \gets i + 2^{d - 1} - 1$
                    \State $\text{temp} \gets e_j$
                    \State $e_j \gets e_k$
                    \State $e_k \gets e_k \bullet \text{temp}$
                \EndFor
            \EndFor
        \EndProcedure
        \\
        \Procedure{Scan}{$[e_1, e_2, \dotsc, e_L]$, $\bullet$}
            \State $\textsc{Reduce}([e_1, e_2, \dotsc, e_L], \bullet)$ \Comment{$L - 1$ $\bullet$ computes.}
            \State $\text{all\_reduced\_out} \gets e_L$ \Comment{Last element of the inclusive scan.}
            \State $\textsc{UpSweep}([e_1, e_2, \dotsc, e_L], \bullet)$ \Comment{$L - 1$ $\bullet$ computes, $L - 1$ swaps.}
            \State \Return $[e_2, \dotsc, e_L, \text{all\_reduced\_out}]$ \Comment{Shift one to the left, append all-reduced output.}
        \EndProcedure
    \end{algorithmic}
    \caption{Blelloch work-efficient parallel (inclusive) scan on a PRAM (for an array of $L$ elements, using a binary operator $\bullet$).}
    \label{alg:scan}
\end{algorithm}

Blelloch work-efficient parallel scan \cite{blelloch1990prefix} for a given array of $L$ elements $e_{1:L}$ using the binary operator in (\ref{eq:recurrence-operator}) is shown in Algorithm~\ref{alg:scan}. We initialize $e_{1:L}$ using (\ref{eq:scan-init}) and run a parallel scan in Algorithm~\ref{alg:scan}. For illustrative purposes, let $L = 4$; now we run the reduce phase as follows:
\begin{align*}
    e_1 &= (\discrete{A}, \discrete{B}x[1]). \\
    e_2 &\gets e_1 \bullet e_2 = (\discrete{A}, \discrete{B}x[1]) \bullet (\discrete{A}, \discrete{B}x[2]) = (\discrete{A}^2, \discrete{A}\discrete{B}x[1] + \discrete{B}x[2]). \\
    e_3 &= (\discrete{A}, \discrete{B}x[3]). \\
    e_4 &\gets e_2 \bullet (e_3 \bullet e_4) \\
    &= e_2 \bullet ((\discrete{A}, \discrete{B}x[3]) \bullet (\discrete{A}, \discrete{B}x[4])) \\
    &=  (\discrete{A}^2, \discrete{A}\discrete{B}x[1] + \discrete{B}x[2]) \bullet (\discrete{A}^2, \discrete{A}\discrete{B}x[3] + \discrete{B}x[4]) \\
    &= (\discrete{A}^4, \discrete{A}^3\discrete{B}x[1] + \discrete{A}^2\discrete{B}x[2] + \discrete{A}\discrete{B}x[3] + \discrete{B}x[4]).
\end{align*}

Next, we store $e_4$ above (as all-reduced output) for later, then set $e_4 = (\I, 0)$ and run the down sweep phase as follows:
\begin{align*}
    e_2 \gets (\I, 0)&; e_4 \gets (\I, 0) \bullet (\discrete{A}^2, \discrete{A}\discrete{B}x[1] + \discrete{B}x[2]) = (\discrete{A}^2, \discrete{A}\discrete{B}x[1] + \discrete{B}x[2]). \\
    e_1 \gets (\I, 0)&; e_2 \gets (\I, 0) \bullet (\discrete{A}, \discrete{B}x[1]) = (\discrete{A}, \discrete{B}x[1]). \\
    e_3 \gets (\discrete{A}^2, \discrete{A}\discrete{B}x[1] + \discrete{B}x[2])&; e_4 \gets (\discrete{A}^2, \discrete{A}\discrete{B}x[1] + \discrete{B}x[2]) \bullet (\discrete{A}, \discrete{B}x[3]) \\
    &\phantom{;  e_4   ~} = (\discrete{A}^3, \discrete{A}^2\discrete{B}x[1] + \discrete{A}\discrete{B}x[2] + \discrete{B}x[3]).
\end{align*}

To generate an inclusive scan, we shift the resulting array one to the left and insert the all-reduced output to the end. As a result, we have the output elements of the parallel scan, $r_{1:4}$, as:
\begin{align*}
    r_1 &= e_2 = (\discrete{A}, \discrete{B}x[1]) = (\discrete{A}, h[1]); \\
    r_2 &= e_3 = (\discrete{A}^2, \discrete{A}\discrete{B}x[1] + \discrete{B}x[2]) = (\discrete{A}^2, h[2]); \\
    r_3 &= e_4 = (\discrete{A}^3, \discrete{A}^2\discrete{B}x[1] + \discrete{A}\discrete{B}x[2] + \discrete{B}x[3]) = (\discrete{A}^3, h[3]); \\
    r_4 &= (\discrete{A}^4, \discrete{A}^3\discrete{B}x[1] + \discrete{A}^2\discrete{B}x[2] + \discrete{A}\discrete{B}x[3] + \discrete{B}x[4]) = (\discrete{A}^4, h[4]).
\end{align*}

Observe that the second entry $b_k$ of $r_k = (A_k, b_k)$ corresponds to the desired $h[k]$. 

\paragraph{Efficiency of a parallel scan.} From Algorithm~\ref{alg:scan}, we note that the scan operation can be performed in $\bigo(T_\bullet\log_2(L))$ time using $L/2$ processors, where $T_\bullet$ is the cost of computing $e_j \bullet e_k$. $T_\bullet$ depends on the structure of $\discrete{A}$; for a general $\discrete{A}$, $T_\bullet$ is dominated by the cost of matrix-matrix multiplication, $\bigo(n^3)$. Hence, the overall cost of a parallel scan for an $L$-length sequence and a general $\discrete{A}$ is $\bigo(n^3 \log_2(L))$.

Furthermore, for $F_\bullet$ FLOPs per $\bullet$ compute, we note the parallel scan to incur $\bigo(F_\bullet L)$ FLOPs, making the work-efficient parallel scan theoretically efficient for a tractable $F_\bullet$. For a general $\discrete{A}$, Algorithm~\ref{alg:scan} results in $\bigo(n^3 L)$ FLOPs.
